# Supplementary material for: No go for a flow
Source: arXiv:2002.07816 ancillary file (2020-05-02)
Supplement: Supplementary file 1 [file Guide_programs.pdf]

# Guide to the programs

Federico Carta<sup>1</sup>, Alessandro Mininno<sup>2</sup>

<sup>1</sup>Deutsches Elektronen-Synchrotron, DESY,  
Notkestraße 85, 22607 Hamburg, Germany

<sup>2</sup>Instituto de Física Teórica IFT-UAM/CSIC,  
C/ Nicolás Cabrera 13-15, Campus de Cantoblanco, 28049 Madrid, Spain  
[federico.carta@desy.de](mailto:federico.carta@desy.de), [alessandro.mininno@uam.es](mailto:alessandro.mininno@uam.es)

## Abstract

Brief description of the programs that have been used. Programs based on [1–5]. The programs work on Linux based operative systems and only with Macaulay2 installed. In case in which Macaulay2 is installed only locally, it is necessary to specify the directory where the executable is.

## Contents

|          |                                 |                          |
|----------|---------------------------------|--------------------------|
| <b>1</b> | <b>GGp_RAC.nb</b>               | <b><a href="#">1</a></b> |
| <b>2</b> | <b>GGp finding UV theory.nb</b> | <b><a href="#">2</a></b> |

## 1 GGp\_RAC.nb

The notebook takes as input two of the following groups

$$A_{n \geq 1} , D_{n \geq 3} , E_6 , E_7 , E_8 , \quad (1.1)$$

and it returns as output an array containing:

- The scaling dimensions of the Coulomb Branch operators.
- The number of masses, i.e. the rank of the flavor symmetry.
- The dimension of the Coulomb Branch.
- The central charges  $a$  and  $c$ .
- The dimension of the Higgs Branch as<sup>1</sup>

$$\dim \text{HB} = 24(c - a) . \quad (1.2)$$

The program needs the name of the simple Lie group, written doubling the letter defining them, e.g.  $AA$  stands for the  $A$  group, and the rank of the group:

---

### Listing 1: Input

---

```
1 G := AA;  
2 n := 5;  
3 Gp := AA;  
4 m := 5;
```

---

The outputs are given in an array through the function  $\text{RAC}[G,n,Gp,m]$ . In the odds components there is the string explaining what is listed in the following even component of the array. As an example, here there is the output for the input in [1](#):

---

<sup>1</sup>In some cases this formula may gives fractional results. In those cases, there is no Higgs branch.

## 2 GGp finding UV theory.nb

Given as an input the rank  $r_{IR}$ , the central charges  $a_{IR}$  and  $c_{IR}$  and the number  $f$  of CB operators with the smallest dimension of any given 4d  $\mathcal{N} = 2$  SCFT  $\mathcal{T}_{IR}$ , the function `UVTheory` computes all the possible UV lagrangian theories which could flow to  $\mathcal{T}_{IR}$  under a Maruyoshi-Song deformation. The functions are based on the works of [3, 5]. The code is then completely general because it needs only information of the IR theory,  $\mathcal{T}_{IR}$  and it will provide an output with all the candidates UV theories as follows. The input of the theory are in 2 and the outputs are given by `UVTheory[r,a,c,f]` of the following form:

$$\begin{aligned}
 & \{ \\
 & \{ \\
 & \quad \{AA_1AA_3AA_5, 53, 80\}, \\
 & \quad \{\}, \\
 & \quad \{\{AA_1, AA_3\}, \{AA_3, AA_5\}\}, \\
 & \quad \{\{AA_1\}, \{AA_3\}, \{AA_5\}\}, \\
 & \quad \{\{y(1, 1, 1) \rightarrow 1, y(2, 1, 1) \rightarrow 1, z(1, 1) \rightarrow 0, z(1, 3) \rightarrow 0, z(1, 4) \rightarrow 0, z(2, 1) \rightarrow 0, \\
 & \quad \quad z(2, 3) \rightarrow 0, z(2, 4) \rightarrow 0, z(3, 1) \rightarrow 8, z(3, 2) \rightarrow 0, z(3, 3) \rightarrow 0, z(3, 4) \rightarrow 0\}\}\} \\
 & \}.
 \end{aligned} \tag{2.1}$$

Listing 2: Input

---

```

1 r := 9;
2 a := 145/24;
3 c := 37/6;
4 f := 3;

```

---

The way in which the output needs to be read is as follows.

Starting from the input, the notebook first select all the possible combination of  $f$  groups whose sum of ranks is equal to  $r$ . Since the rank is preserved during the RG flow [3], the UV theory is then given by  $f$  groups whose sum of the ranks given by  $r$ . This selection is done through 3 and the result is stored in different functions, such as

`NTuples` and `EffListofgroups`. This is the function that takes most of the time of the simulation. In fact, it can take days to compute all possible combinations of a single configuration. There should not be problem with the saturation of the RAM because the function saves a combination of groups only if such combination satisfies the condition that the rank is equal to  $r$ . The problem is only on the large amount of possibilities when  $f$  is large (usually larger than 3). Using `GroupNvNh` we are able to obtain also the total number of vector multiplet for each combinations of groups, computing the dimensions of the groups using `dimGr`, and the number of hypermultiplets, using `Nh` and the inputs  $a$  and  $c$ , as explained, for instance, in [3]. For any combination of groups, the number of vector multiplets and hypermultiplets is stored in an array given by `GroupNvNh`.

Now it is time to check which combinations of groups is a candidate for a conformal  $\mathcal{N} = 2$  SCFT in the UV. There are three main functions that select the possible single factors, pairs and triplets of groups that are allowed by [5]. For each of these categories it is associated a representation and its dimension. Following [5], a single group admits hypermultiplets in different kind of representations. Moreover these hypers can be full or half. Looking at table 1 of [5], it is possible to count all the possible representations that all the groups can have and there are 12 of them. It is worth to say that not all the groups admit all the 12 different representations. This is just a computational trick to have an easy way to store the dimensions of each representation and to access them in a fast way. Usually, in other contexts, this dictionary that we have created can be thought as an "Hash table". At each group, it is then associated an array of 12 components each of them corresponding to a possible representation. If the group admits such representation, the component of the array is modified by the dimension of the group under that representation, otherwise the component is kept zero. The components of the array are associated at the following representations:

1. Fundamental / Vector representation.
2. Antisymmetric representation.
3. Symmetric representation.
4. Adjoint representation.

5. 3-index antisymmetric representation.
6. S - spinorial representation.
7. C - conjugate spinorial representation.
8. 16 dimensional representation.
9. 27 dimensional representation.
10. 56 dimensional representation.
11. 26 dimensional representation.
12. 7 dimensional representation.

It is now clear that not all the groups can have all these representations. Some of them are specific for some exceptional group and they are not allowed for other. The function `SingleNodeDimList` checks each group for the combination given by `GroupNvNh` and export an array containing the group and the 12 component array where only the component associated to the allowed representation are different to zero and, in particular, they are set equal to the dimension of such representation for the hypers (half or full) in that representation. The function `DoubleNodeDimList` repeats what the previous function did but for any pair that can be formed by the combination given by `GroupNvNh`. The output is an containing the element of each pair with associated the 12 dimensional array where the only non zero components are those ones associated to the allowed representation. Moreover there is a matrix  $12 \times 12$  where there are all the possible dimensions that a bifundamental hypermultiplet can have. Finally, the function `TripleNodeDimList` does the same play for triplets. The output contains each element of the triplet, associated to the 12 dimensional array and finally a matrix  $12 \times 12 \times 12$  with all the possible dimensions of the representation that a trifundamental hypermultiplet can have.

Each hypermultiplet in a specific representation contributes differently to the Beta function of each gauge group. The different weights are programmed in the function `Betafuncoeff`. Following [5], the sum of all the hypermultiplets in their representation, weighted by their contribution to the beta function, needs to be equal to twice

the dual Coxeter number of the group. The dual Coxeter number for each group is in `Coxetervalue`.

Now we come to the most important function of the notebook, `Numberhyperpernode`. For any  $r$  and  $f$ , there can be many combinations of groups. We call the number of combination `lengthgroupnvnh`. For each one of these combinations, there can be a different number of triplets, pairs and single groups. We, now define three variables  $X$ ,  $Y$  and  $Z$ . They are arrays defined as:

1.  $X$  is a matrix  $N_{\text{triplets}} \times 12 \times 12 \times 12$ , where  $N_{\text{triplets}}$  is the number of triplets that satisfies the constraints given by [5].
2.  $Y$  is a matrix  $N_{\text{pairs}} \times 12 \times 12$ , where  $N_{\text{pairs}}$  is the number of pairs that satisfies the constraints given by [5].
3.  $Z$  is a matrix with  $N_{\text{single}} \times 12$ , where  $N_{\text{single}}$  is the number of single groups that satisfies the constraints given by [5].

The  $X$  matrix is associated to the hypermultiplets in a triplet representation, where there are  $12 \times 12 \times 12$  possibilities. The  $Y$  matrix is associated to the hypermultiplets in a double representation, where there are  $12 \times 12$  possibilities. The  $Z$  array is associated to the hypermultiplet in a single representation, where there are 12 possibilities.

Now, let us take  $Y$  as example, to see how the variables are set. In principle,  $Y = y_{i,j,l}$ , where  $i = 1, \dots, N_{\text{pairs}}$ ,  $j, l = 1, \dots, 12$ . and  $y_{i,j,l}$  is the variable associated to the  $i$ -th hyper in the double representation  $(j, l)$ , where  $j$  is the index associated to the possible representations of the first element of the pair,  $G$  and  $l$  is the index associated to the possible representations second element of the pair,  $G'$ . So, there can be  $y_{i,j,l}$  hypermultiplets contributing  $\dim G$  to the beta function of  $G'$  weighted by `Betafuncoeff` for the group  $G'$  and vice-versa.

Repeating this discussion also for  $X$  and  $Z$ , the program solves a system of equations where the sum of all the variables is equal to the total number of hypermultiplets that there are in this combination and the contribution of the sum of hypermultiplets charged under a group is equal to twice the dual Coxeter index of the group.

We are now able to interpret the output in Eq. (2.1). For a group  $AA_1AA_3AA_5$ , there are not allowed triplets, so  $X = 0$ , there are two possible pairs, so  $Y = y_{i,j,l}$  with

$i = 1, 2$  and  $j, l = 1, \dots, 12$  and three allowed single groups, so  $Z = z_{k,j}$  with  $k = 1, 2, 3$  and  $j = 1, \dots, 12$ . The components  $j$  and  $l$  represent the kind of representations that an hypermultiplet can have, following the previous list. So there is 1 bifundamental hypermultiplet for each pair, and 8 hypermultiplets charged under  $A_5$  in the fundamental representation.

Listing 3: SelectTuples code by Sander Huisman

---

```

1 ClearAll[ SelectTuples ]
2 SelectTuples [ list_List , n_Integer?NonNegative,crit_,m_:\[Infinity] ]:=Module{ {len=Length[list],vars
   , val , its , result ,found=0},
3 vars=Table[Unique["i"],n];
4 its={ #,len}&/@vars;
5 result=Reap[
6 Do[
7 val=Part[list , vars ];
8 If [ TrueQ[crit[val ]],
9 found++;
10 If [found>m,Break[]];
11 Sow[val];
12 ]
13 ,
14 Evaluate[Sequence@@its]
15 ];
16 ];
17 First [ result  [[2]],{}}
18 ]
19 SelectTuples [ list : { _List ...}, crit_ , m_:\[Infinity] ]:=Module{ {n=Length[list],lens=Length/@list,
   vars,val , its , result ,found=0},
20 vars=Table[Unique["i"],n];
21 its=Transpose[{vars,lens}];
22 result=Reap[
23 Do[
24 val=MapThread[Part,{list,vars}];
25 If [ TrueQ[crit[val ]],
26 found++;
27 If [found>m,Break[]];
28 Sow[val];
29 ]

```

```

30 ,
31 Evaluate[Sequence@@@its]
32 ];
33 ];
34 First [ result [[2]], {}]
35 ];

```

---

## References

- [1] D. Xie, *General Argyres-Douglas Theory*, *JHEP* **01** (2013) 100, [[arXiv:1204.2270](#)].
- [2] S. Cecotti, A. Neitzke, and C. Vafa, *R-Twisting and 4d/2d Correspondences*, [arXiv:1006.3435](#).
- [3] S. Giacomelli, *Infrared enhancement of supersymmetry in four dimensions*, *JHEP* **10** (2018) 041, [[arXiv:1808.00592](#)].
- [4] K. Maruyoshi and J. Song, *Enhancement of Supersymmetry via Renormalization Group Flow and the Superconformal Index*, *Phys. Rev. Lett.* **118** (2017), no. 15 151602, [[arXiv:1606.05632](#)].
- [5] L. Bhardwaj and Y. Tachikawa, *Classification of 4d  $N=2$  gauge theories*, *JHEP* **12** (2013) 100, [[arXiv:1309.5160](#)].
